# Supplementary material for: Experimental determination of circuit equations
Source: arXiv:1309.4848 ancillary file (2013-09-19)
Supplement: Supplementary file 1 [file SupplementaryMaterials_ModelParameters.pdf]

# Calculating model parameters

This supplementary material presents an algorithm for calculating the parameters of the network model for a circuit of resistors. The network equations describing such a circuit with $N$ nodes connected to a dc power supply are,

$$0 = \sum_j A_{ij} \left( V_j - V_j^{(o)} \right), \tag{1}$$

for $i, j = 1, 2, \ldots, N$. Here, $\mathbf{A}$ is an $N$x$N$ matrix, and $\mathbf{V^{(o)}}$ is an $N$-element vector containing the node potentials of the unperturbed circuit. The defining feature of the network model is that these constants are determined by experiment.

In order to calculate the parameters, $N + 1$ experiments need to be performed. Measuring the node potentials for the unperturbed circuit directly determines $\mathbf{V^{(o)}}$. The remaining experiments involve fixing the potential of a single node and measuring the potentials of the $N - 1$ remaining nodes. This is done for each node. In this work, we set the fixed potential to be zero; however, this is not required, and any convenient potential can be used.

The procedure for calculating the model parameters will be demonstrated on a circuit with three nodes for simplicity. It can be extended easily to larger circuits. During a measurement of the unperturbed circuit, the equations describing the node potential values are simply Eqs. (1), *i.e.,*

$$0 = A_{11} \left( V_1 - V_1^{(o)} \right) + A_{12} \left( V_2 - V_2^{(o)} \right) + A_{13} \left( V_3 - V_3^{(o)} \right) \tag{2a}$$

$$0 = A_{21} \left( V_1 - V_1^{(o)} \right) + A_{22} \left( V_2 - V_2^{(o)} \right) + A_{23} \left( V_3 - V_3^{(o)} \right) \tag{2b}$$

$$0 = A_{31} \left( V_1 - V_1^{(o)} \right) + A_{32} \left( V_2 - V_2^{(o)} \right) + A_{33} \left( V_3 - V_3^{(o)} \right). \tag{2c}$$

Clearly, the potentials $\mathbf{V^{(o)}}$ satisfy these equations.

The remaining experiments involve fixing a single node potential to zero by grounding. When node one is grounded, for example, the equation describing its behavior is no longer valid because the node is under external control and no longer influenced by the others. In such a situation, the node potentials of the remaining nodes will be modified from their normal values. The new potentials, when measured, are $\mathbf{V^{(1)}} = \left[ V_1^{(1)}, V_2^{(1)}, V_3^{(1)} \right]$, with $V_1^{(1)} = 0$. The equations corresponding to such an experiment can be written

as,

$$V_1^{(1)} = 0 \tag{3a}$$

$$0 = A_{21}\left(V_1^{(1)} - V_1^{(o)}\right) + A_{22}\left(V_2^{(1)} - V_2^{(o)}\right) + A_{23}\left(V_3^{(1)} - V_3^{(o)}\right) \tag{3b}$$

$$0 = A_{31}\left(V_1^{(1)} - V_1^{(o)}\right) + A_{32}\left(V_2^{(1)} - V_2^{(o)}\right) + A_{33}\left(V_3^{(1)} - V_3^{(o)}\right). \tag{3c}$$

Next, node two is grounded to obtain the potentials $\mathbf{V^{(2)}}$ and the equations

$$0 = A_{11}\left(V_1^{(2)} - V_1^{(o)}\right) + A_{12}\left(V_2^{(2)} - V_2^{(o)}\right) + A_{13}\left(V_3^{(2)} - V_3^{(o)}\right) \tag{4a}$$

$$V_2^{(2)} = 0 \tag{4b}$$

$$0 = A_{31}\left(V_1^{(2)} - V_1^{(o)}\right) + A_{32}\left(V_2^{(2)} - V_2^{(o)}\right) + A_{33}\left(V_3^{(2)} - V_3^{(o)}\right). \tag{4c}$$

Grounding node three generates,

$$0 = A_{11}\left(V_1^{(3)} - V_1^{(o)}\right) + A_{12}\left(V_2^{(3)} - V_2^{(o)}\right) + A_{13}\left(V_3^{(3)} - V_3^{(o)}\right) \tag{5a}$$

$$0 = A_{21}\left(V_1^{(3)} - V_1^{(o)}\right) + A_{22}\left(V_2^{(3)} - V_2^{(o)}\right) + A_{23}\left(V_3^{(3)} - V_3^{(o)}\right) \tag{5b}$$

$$V_3^{(3)} = 0. \tag{5c}$$

These are all the equations needed to calculate the model parameters. We can now collect the equations containing similar elements of $\mathbf{A}$. For example, Eqs. (2a), (4a), (5a), all contain the first-row elements. These can be written in matrix form, *i.e.,*

$$\begin{bmatrix} 0 \\ 0 \\ 0 \end{bmatrix} = \begin{pmatrix} V_1^{(o)} - V_1^{(o)} & V_2^{(o)} - V_2^{(o)} & V_3^{(o)} - V_3^{(o)} \\ V_1^{(2)} - V_1^{(o)} & V_2^{(2)} - V_2^{(o)} & V_3^{(2)} - V_3^{(o)} \\ V_1^{(3)} - V_1^{(o)} & V_2^{(3)} - V_2^{(o)} & V_3^{(3)} - V_3^{(o)} \end{pmatrix} \begin{bmatrix} A_{11} \\ A_{12} \\ A_{13} \end{bmatrix}. \tag{6}$$

The matrix contains the data collected from experiment. The unperturbed data has been included in the first equation for the moment. If a computer, *e.g.,* with software such as Matlab, is used to solve this system of homogeneous equations for $[A_{11}, A_{12}, A_{13}]$, it will return a vector of zeros, which is not the desired solution, of course. A few manipulations are necessary to avoid this. First, the $V_1^{(o)}$ terms in the left column are moved to the other

side of the equations. The remaining elements of the top row are simplified by inserting a value of zero. This results in,

$$\begin{bmatrix} V_1^{(o)} \\ V_1^{(o)} \\ V_1^{(o)} \end{bmatrix} = \begin{pmatrix} V_1^{(o)} & 0 & 0 \\ V_1^{(2)} & V_2^{(2)} - V_2^{(o)} & V_3^{(2)} - V_3^{(o)} \\ V_1^{(3)} & V_2^{(3)} - V_2^{(o)} & V_3^{(3)} - V_3^{(o)} \end{pmatrix} \begin{bmatrix} A_{11} \\ A_{12} \\ A_{13} \end{bmatrix}. \tag{7}$$

The first equation produces $A_{11} = 1$, and the remaining parameters can now be calculated.

A similar procedure can be followed to calculate the remaining rows of $\mathbf{A}$. As discussed in the main text, for a circuit of resistors, the equations generated by the network method are the same as those obtained using Kirchhoff's laws.

We have included, in the Supplementary Materials, a Matlab function which automates the calculation of the $\mathbf{A}$ matrix. It requires a two inputs, the total number of nodes ($N$) and the matrix of data obtained by experiment. The matrix should have the form,

$$\begin{pmatrix} V_1^{(1)} & V_2^{(1)} & V_3^{(1)} & \cdots & V_N^{(1)} \\ V_1^{(2)} & V_2^{(2)} & V_3^{(2)} & \cdots & V_N^{(2)} \\ \vdots & \vdots & \vdots & \ddots & \vdots \\ V_1^{(N)} & V_2^{(N)} & V_3^{(N)} & \cdots & V_N^{(N)} \\ V_1^{(o)} & V_2^{(o)} & V_3^{(o)} & \cdots & V_N^{(o)} \end{pmatrix}. \tag{8}$$

Note the position of the unperturbed data. It is included at the bottom of the matrix.
